# Supplementary material for: Melting a granular glass by cooling
Source: arXiv:1210.1945 source file (2013-02-05)
Supplement: Supplementary file 1 [file supplMat.pdf]

# Supplementary material: Melting a granular glass by cooling

Jan Plagge and Claus Heussinger
*Institute for Theoretical Physics, Georg-August University of Göttingen, Friedrich-Hund Platz 1, 37077 Göttingen*

## I. SINGLE-PARTICLE OSCILLATION WITH AND WITHOUT FRICTION

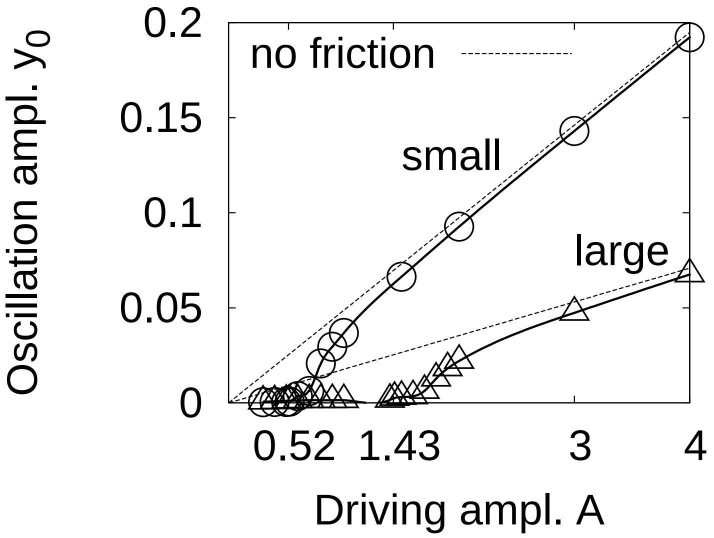


FIG. 1: Oscillation amplitudes of independent (large or small) particles as a function of driving amplitude $A$ on a frictional surface. Below the Coulomb threshold ($A_s = 0.52$ for the small and $A_l = 1.43$ for the large particles) the particles remain immobile on the surface. For large driving amplitudes the particles behave as without friction.

## II. STICK-SLIP BEHAVIOR

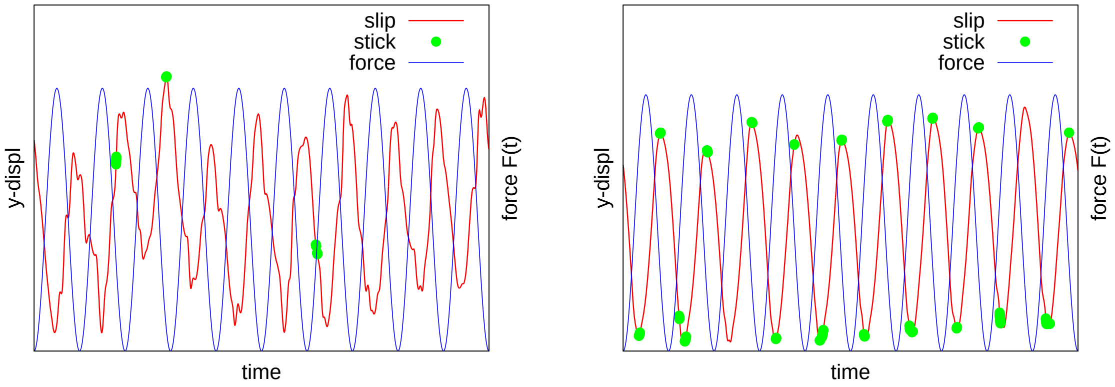


FIG. 2: Illustration of the force-induced oscillations $y(t)$ of a small particle in the glassy (left) and the re-entrance fluid phase (right). In the glassy phase the forcing is out-of phase with the displacement and stick events are seldom. In the fluid phase the forcing is essentially in phase with the velocity. The particle sticks to the surface quite regularly.

## III. RELAXATION OF COLLISIONAL MOMENTUM

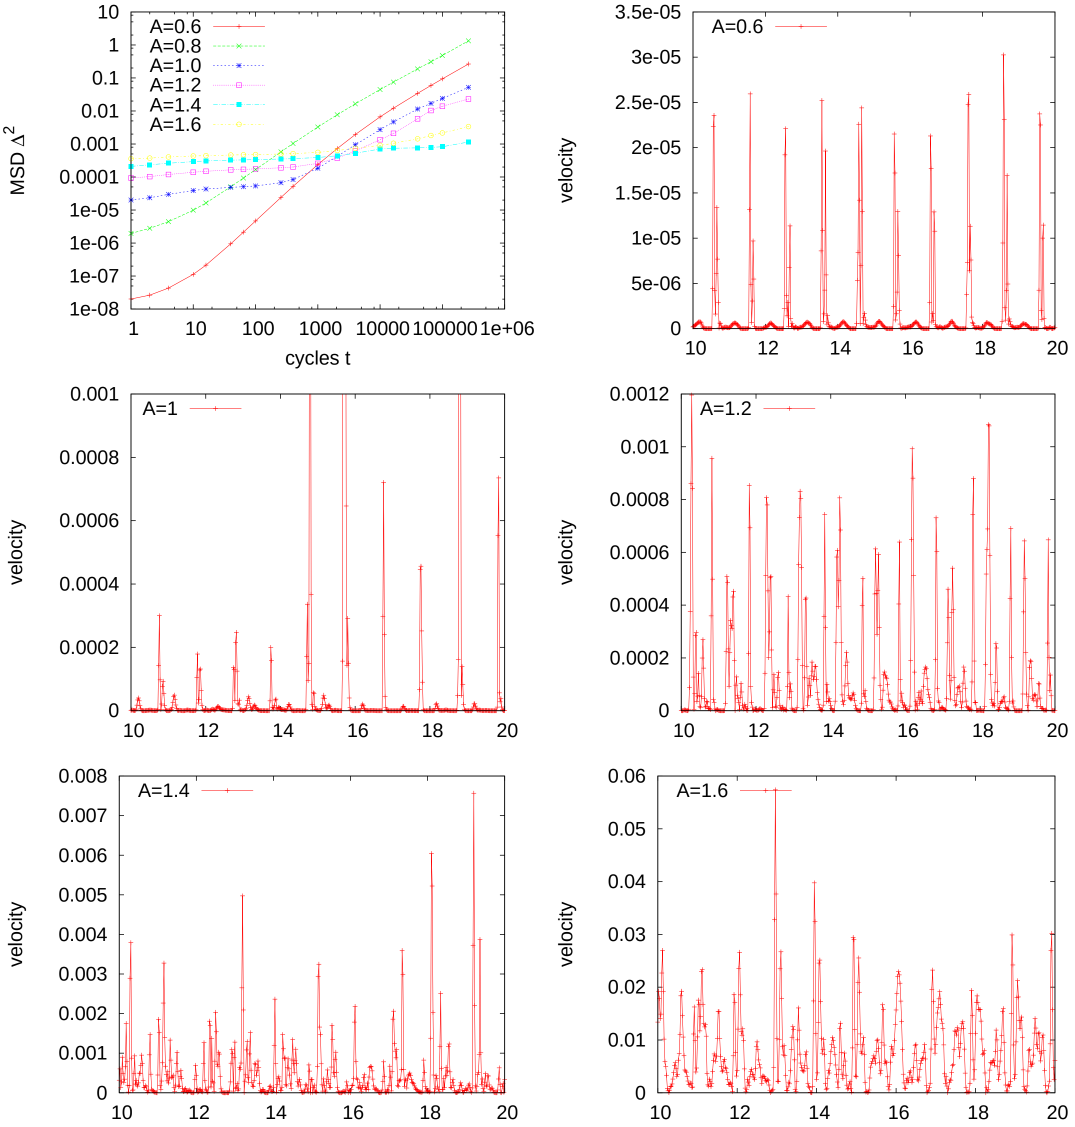


FIG. 3: In this system only the small particles are driven. The large particles therefore only move because they receive kicks from the small particles. Surface friction acts on the small particles, but large particles feel the linear viscous force. The MSD displays the same re-entrance melting transition as presented in the manuscript. The onset of re-entrance melting corresponds to the situation, where momentum is dissipated sufficiently fast. In the fluid phase particles can therefore come to rest in between collisions. Shown are the magnitude of the velocities of a large particle during the course of ten force oscillations.

## IV. SLOW EVOLUTION OF THE CAGE

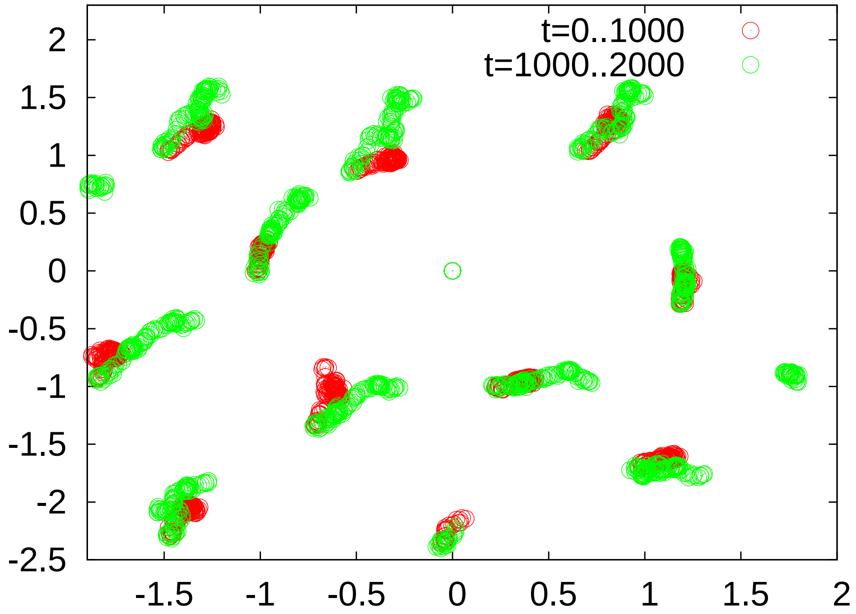


FIG. 4: Illustration of the evolution of a cage over the time-scale of $t = 2000$ force oscillations. Positions of surrounding particles are measured in the rest-frame of the central particle. The cage continuously evolves/deforms as the surrounding particles move relative to the cage center. A drift motion of an intact cage should not lead to such motion.
